# Supplementary material for: Processing stationary noise: model and parameter selection in variational methods
Source: arXiv:1307.4592 source file (2013-07-17)
Supplement: Supplementary file 1 [file Notes_Supplementaires.tex]

\subsection{Polynomial behaviors}

We further assume that:
$$
\psi(x)\leq \frac{M}{|x|^\beta}.
$$
and 
$$
\psi(x)\geq \frac{m}{|x|^\beta}.
$$
where $\beta,M,m>0$ and $|x|>\epsilon>0$. 

We may wonder which $\beta$ ensures convergence to a Normal distribution as $n\rightarrow+\infty$. 
Since we assume that $\Lambda$ is an i.i.d. random vector with $0$ mean, convergence will occur for any choice of the marginals of $\Lambda$. 
We thus only look for a condition on $\beta$.

Let us denote:
$$
f(R)=\frac{\int_{B(0,R) \backslash B(0,\epsilon)}|\psi|^3(x) dx}{\left(\int_{B(0,R)\backslash B(0,\epsilon)}|\psi|^2(x) dx\right)^{3/2}}.
$$
Note that $\frac{\sum_{i=1}^n \rho_i}{(\sum_{i=1}^n \sigma_i^2)^{3/2}}$ in equation \eqref{eq:Berry} is just a Riemann approximation of $f(R)$ for a certain $R$.

The integrals can be computed explicitely using polar coordinates: 
\begin{align*}
\int_{B(0,R)\backslash B(0,\epsilon)}|\psi|^2(x) dx &\geq 2\pi m^2\int_{\epsilon}^R  \frac{1}{r^{2\beta}} r dr \\ 
&= 2\pi m^2 \left[\frac{r^{2-2\beta}}{2-2\beta}\right]_{\epsilon}^{R}
\end{align*}
This quantity will tend to $+\infty$ if $2-2\beta>0$, i.e. $\beta<1$. In that case:
$$
\left(\int_{B(0,R)\backslash B(0,\epsilon)}|\psi|^2(x) dx \right)^{3/2}\stackrel{R=+\infty}{\sim} R^{3-3\beta}c.
$$
with $c>0$. Similarly:
\begin{align*}
\int_{B(0,R)\backslash B(0,\epsilon)}|\psi|^3(x) dx &\leq 2\pi M^3\int_{\epsilon}^R  \frac{1}{r^{3\beta}} r dr \\ 
&= 2\pi M^3 \left[\frac{r^{2-3\beta}}{2-3\beta}\right]_{\epsilon}^{R}.
\end{align*}

Looking at these expressions, we get that the upper bound in \eqref{eq:Berry} goes to $0$ as long as $\beta<1$.
Finally, we get the result:

\begin{center}
 For any kernel $\psi$ decaying to $0$ slowlier than $\frac{1}{|x|}$, the noise distribution is Gaussian whatever the marginals of $\Lambda$ (for an infinite number of pixels).
\end{center}

Je ne sais pas trop ce qui se passe lorsque le filtre peut prendre des valeurs positives et n\'egatives. Par exemple pour l'image du Baboon j'ai utilis\'e un sinus cardinal.

\subsection{The case of a Bernoulli-Uniform noise + a Gaussian kernel}

This is the kind of distribution which would lead to ``sparse'' signals. 
\footnote{I guess that Bernoulli-Gaussian or Bernoulli-Laplace distributions would lead to the same kinds of bound.} 

It satisfies:
$$
p(\Lambda(y)\neq 0)=\alpha.
$$
$$
p(\Lambda(y)=0)=1-\alpha.
$$
and 
$$
\Lambda(y)|\Lambda(y)\neq 0 \sim U([-1,1]).
$$

For this distribution, we have:
$$
\E(\Lambda(y))=0,
$$
$$
\sigma^2=\E(\Lambda^2(y))=\alpha \int_{-1}^1x^2dx = \frac{2}{3}\alpha,
$$
and
$$
\rho=\E(|\Lambda(y)|^3)=2\alpha \int_{0}^1x^3dx = \frac{\alpha}{2}.
$$

Now, let us set:
$$
\psi(x_1,x_2)=\frac{1}{2\pi \sigma_1\sigma_2}\exp\left( - \frac{x_1^2}{\sigma_1^2}- \frac{x_2^2}{\sigma_2^2}\right).
$$
This corresponds to what is used in our experiments.

We want to assess the distance from $B(0)$ to the Normal distribution. We have:
$$
\E(\Lambda(y)\psi(x-y))=0,
$$
$$
\sigma^2(x-y)=\E(\Lambda^2(y)\psi(x-y))=\frac{2}{3}\alpha \psi^2(x-y),
$$
and
$$
\rho(x-y)=\E(|\Lambda(y)\psi(x-y)|^3)=\frac{\alpha}{2}|\psi|^3(x-y).
$$

These quantities can be replaced in \eqref{eq:Berry} leading to:
$$
\|F_n-\Phi\|_\infty\leq \frac{C_1}{\sqrt{\alpha}} \frac{\sum_{x} |\psi(x)^3|}{(\sum_{x} \psi(x)^2)^{3/2}}.
$$
where $F_n$ is the distribution function of $B(0)$ and $C_1=\frac{1}{2}C_0\left( \frac{2}{3}\right)^{-3/2}$.

We use the approximations:
$$
\sum_{x} |\psi|^3(x-y)\simeq \int_{\mathbb{R}^2}|\psi|^3(x-y)dy_1dy_2 
$$
and 
$$
\sum_{y_1,y_2} \psi^2(y_1,y_2)\simeq \int_{\mathbb{R}^2}\psi^2(y_1,y_2)dy_1dy_2. 
$$
These integrals can be computed exactly:
$$
\int_{\mathbb{R}^2}|\psi|^3(x-y)dy_1dy_2=\frac{1}{12\pi \sigma_1^2\sigma_2^2}
$$
and
$$
\int_{\mathbb{R}^2}|\psi|^2(x-y)dy_1dy_2=\frac{1}{4\pi \sigma_1\sigma_2}.
$$

Overall we get that (sauf erreur):
\begin{equation}
\|F_n-\Phi\|_\infty\leq \frac{C_2}{\sqrt{\alpha}} \sqrt{\frac{\pi}{\sigma_1\sigma_2}}. 
\end{equation}

where $C_2=\frac{2}{3}C_1$. Looking at this expression we see that:
\begin{itemize}
 \item In the case $\alpha=1$, $\Lambda$ has a uniform distribution. This analysis thus covers the cases of white uniform processes and the class of Bernoulli-Uniform signals.
 \item The sparsest the signal (i.e. the smaller $\alpha$), the least accurate the Gaussian approximation. 
However, this does not look too bad since there is a $\sqrt{\cdot}$ on $\alpha$. 
 \item Both $\sigma_1$ and $\sigma_2$ should be ``far'' from $0$ to get a good approximation. This is not too good... 
 \item It could be interesting to evaluate these values numerically for typical values of $\sigma_1$ and $\sigma_2$.
\end{itemize}

%%%%%%%%%%%%%%%%%%%%%%%%%%%%%%%%%%%%%%%%%%%%%%%%%%%%%%%%%%%%%%%%%%%%%%%%%%%%%%%%%%%%%%%%%%%%%%%%%%%%%%%%%%%%%%%%%%%%%%%%%%%%%%%%%%%%%

\subsection{1D}

Let $(\psi(k))_{k\in \N^*}$ denote a sequence of kind $\psi(k)=k^m, \ m\in \N$.
The truncated serie $\sum_{k=1}^N \psi(k)^m$ satisfies:
$$\sum_{k=1}^N \psi(k)^m\sim C(m) N^{m+1}$$
where $C(m)>0$ only depends on $m$.

Thus by denoting 
$$
f(N)=\frac{\sum_{k=1}^N \psi(k)^3}{(\sum_{k=1}^N \psi(k)^2)^{3/2}},
$$
we get:
$$
\lim_{N\rightarrow +\infty} f(n) = \lim_{N\rightarrow +\infty} \frac{C(3m+1) N^{3m+1}}{ C(2m+1) N^{3m+3/2}}=0.
$$
We can thus state the following result:
\begin{proposition} 
Let $\lambda_n$ denote an i.i.d. random vector of size $n$. We assume that the marginals of $\lambda_n$ have finite variance and third order moments. 
Let $\psi_n=(\psi(k))_{k=1}^n$.
For all sequences of kind $\psi(k) = k^m$, $m \in \N$, the random variable:
$$
b_n=\lambda_n\times \psi_n
$$
converges in law to a gaussian vector $\mathcal{N}(0,\mathcal{F}^{-1}\mathop{diag}(|\hat \psi|^2) \mathcal{F})$ as $n$ goes to infinity.
\end{proposition}

By a similar reasoning obtained by comparing the serie to an integral, we get:
\begin{proposition} 
For all kernels satisfying $|\psi(k)|\sim k^\alpha$, $\alpha \geq -1/2$, the random variable:
$$
b_n=\lambda_n\times \psi_n
$$
converges in law to a gaussian $\mathcal{N}(0,\mathcal{F}^{-1}\mathop{diag}(|\hat \psi|^2) \mathcal{F})$.
\end{proposition}

Looking at the above result, it seems possible that $f(n)$ goes to $0$ as long as $\sum_{k=1}^N \psi(k)^2$ diverges. 
This would be nice!

\subsection{What happens in higher dimensions}
